# Supplementary material for: Optical properties and electronic correlations in La$_3$Ni$_2$O$_7$ bilayer nickelates under high pressure
Source: arXiv:2401.04258 ancillary file (2024-09-02)
Supplement: Supplementary file 1 [file SI.pdf]

# Optical properties and electronic correlations in $La_3Ni_2O_7$ bilayer nickelates under high pressure
# Supplementary Information

Benjamin Geisler,[1,2] Laura Fanfarillo,[3] James J. Hamlin,[1] Gregory R. Stewart,[1] Richard G. Hennig,[2,4] and P.J. Hirschfeld[1]

[1]*Department of Physics, University of Florida, Gainesville, Florida 32611, USA*

[2]*Department of Materials Science and Engineering, University of Florida, Gainesville, Florida 32611, USA*

[3]*Istituto dei Sistemi Complessi (ISC-CNR), Via dei Taurini 19, I-00185 Rome, Italy*

[4]*Quantum Theory Project, University of Florida, Gainesville, Florida 32611, USA*

## I. CORRELATION DEPENDENCE OF THE ELECTRONIC STRUCTURE

Supplementary Figure 1 tracks the correlation dependence of the electronic structure of $La_3Ni_2O_7$. Particularly noteworthy are the fractional occupation of the lower Ni $3d_{z^2}$ states observed for $U \leq 2$ (with the surprising exception of $U = 0$ at optimized geometry) even without external pressure, as well as the fractional occupation of the upper Ni $3d_{z^2}$ states found for $U \geq$ 5-6 eV. The fully occupied Ni $t_{2g}$ manifold shifts to lower energies with increasing $U$, enhancing its hybridization with the O $2p$ states located predominantly below $\sim -2$ eV. Simultaneously, the Ni $3d_{x^2-y^2}$ states are pushed to higher energies, reducing their occupation and involvement in the Fermi surface, as well as their hybridization with the Ni $3d_{z^2}$ orbitals around the $M$ point. This shows that $U$ considerably impacts the Ni $e_g$ orbital polarization in this system.

Moreover, we can deduce from the band structure overview that the recently suggested pressure-driven topological transition of the Fermi surface, characterized by an emerging hole pocket of Ni $3d_{z^2}$ character [1–7] and possibly accompanied by a strong $s^{\pm}$ superconducting pairing [3, 4, 6–8], is limited to a relatively small window of $U \sim$ 3-4 eV. Intriguingly, our analysis of the optical spectrum establishes that an appropriate $U$ is indeed located in this interval. We note that *hole* doping in $La_3Ni_2O_7$, e.g., due to oxygen excess or La-Sr substitution, facilitates the formation of the Ni $3d_{z^2}$ hole pocket and hence may be an interesting strategy to reduce the critical pressure.

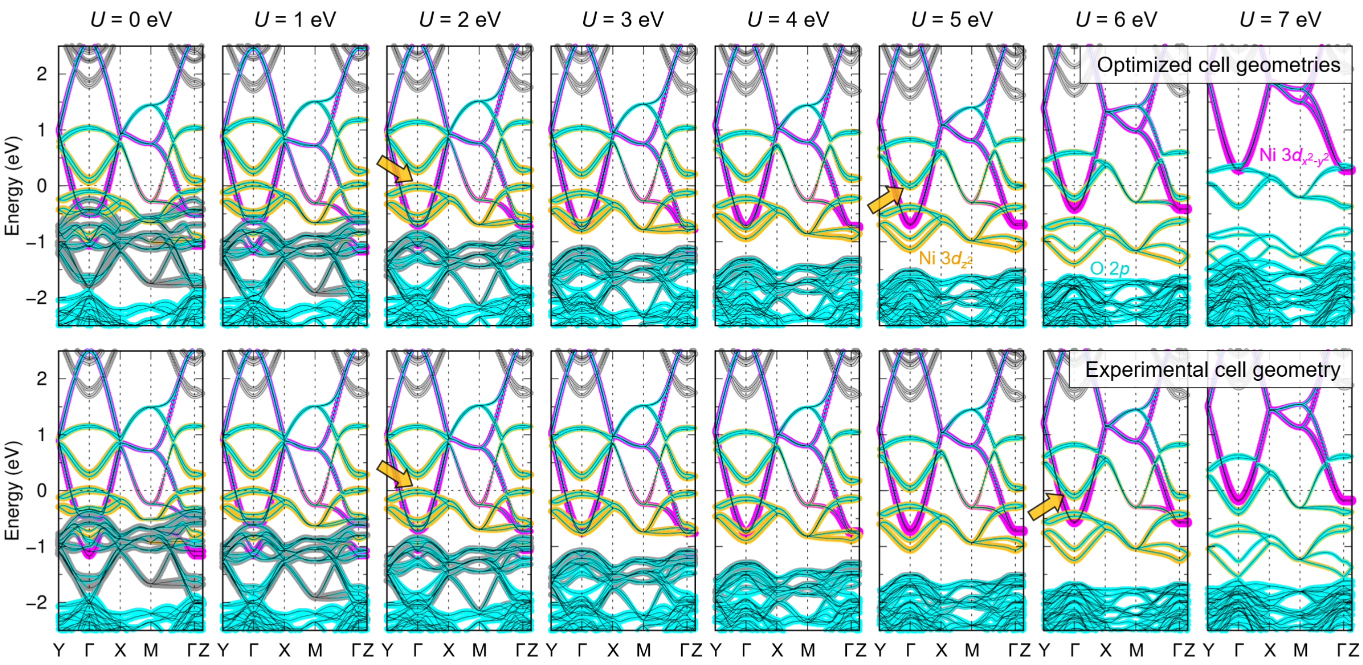


Supplementary Figure 1. Correlation dependence of the band structure of $La_3Ni_2O_7$ at ambient pressure for optimized cell geometries (top row) and the experimental [9] cell geometry (bottom row). The colors represent the orbital character, consistent with Fig. 1 in the main text. The orange arrows mark the fractional occupation of the lower Ni $3d_{z^2}$ states for $U \leq 2$ and of the upper Ni $3d_{z^2}$ states for $U \geq$ 5-6 eV.

## II. DRUDE CONTRIBUTION TO THE OPTICAL CONDUCTIVITY

Supplementary Table I provides predictions of the plasma frequencies for the systems considered in this work, even though our focus is on the interband transitions. Overall, the data presents a strong in-plane versus out-of-plane anisotropy, reflecting the layered crystal structure. In $La_3Ni_2O_7$, external pressure increases $\omega_p^2$ and thus the spectral weight of the Drude peak significantly. In contrast, explicit oxygen vacancies reduce the plasma frequency. The infinite-layer compound $NdNiO_2$ exhibits the highest in-plane $\omega_p^2$. Moreover, the high $\omega_{p,zz}^2$ is indicative of the substantial inter-layer coupling via the Nd $5d$ states [10].

Supplementary Table I. Plasma frequency squared $\omega_{p,\alpha\alpha}^2$ ($eV^2$) as predicted by DFT+$U$ for the systems shown in Figs. 1, 3, and 5 of the main text.

| System | $\omega_{p,xx}^2$ | $\omega_{p,yy}^2$ | $\omega_{p,zz}^2$ |
|---|---|---|---|
| $La_3Ni_2O_7$ | 9.53 | 9.97 | 0.019 |
| $La_3Ni_2O_{6.75}$ (explicit $V_O$) | 8.89 | 8.13 | 0.0 |
| $La_3Ni_2O_7$ ($p$ = 30 GPa) | 16.65 | 16.65 | 0.20 |
| $La_3Ni_2O_7$ ($p$ = 50 GPa) | 15.74 | 15.74 | 0.31 |
| $La_3Ni_2O_7$ (1-3 stacking) | 9.61 | 10.25 | 0.007 |
| $La_4Ni_3O_{10}$ | 12.76 | 14.97 | 0.14 |
| $La_3Ni_2O_6$ | 9.49 | 10.39 | 0.0 |
| $NdNiO_2$ | 25.74 | 25.74 | 9.43 |


[1] Sun, H. *et al.* Signatures of superconductivity near 80 K in a nickelate under high pressure. *Nature* **621**, 493–498 (2023).

[2] Luo, Z., Hu, X., Wang, M., Wú, W. & Yao, D.-X. Bilayer two-orbital model of $La_3Ni_2O_7$ under pressure. *Phys. Rev. Lett.* **131**, 126001 (2023).

[3] Gu, Y., Le, C., Yang, Z., Wu, X. & Hu, J. Effective model and pairing tendency in bilayer Ni-based superconductor $La_3Ni_2O_7$. Preprint at https://arxiv.org/abs/2306.07275 (2023).

[4] Yang, Q.-G., Wang, D. & Wang, Q.-H. Possible $s_\pm$-wave superconductivity in $La_3Ni_2O_7$. *Phys. Rev. B* **108**, L140505 (2023).

[5] Lechermann, F., Gondolf, J., Bötzel, S. & Eremin, I. M. Electronic correlations and superconducting instability in $La_3Ni_2O_7$ under high pressure. *Phys. Rev. B* **108**, L201121 (2023).

[6] Liu, Y.-B., Mei, J.-W., Ye, F., Chen, W.-Q. & Yang, F. $s^\pm$-wave pairing and the destructive role of apical-oxygen deficiencies in $La_3Ni_2O_7$ under pressure. *Phys. Rev. Lett.* **131**, 236002 (2023).

[7] Zhang, Y., Lin, L.-F., Moreo, A., Maier, T. A. & Dagotto, E. Structural phase transition, s±-wave pairing, and magnetic stripe order in bilayered superconductor $La_3Ni_2O_7$ under pressure. *Nat. Commun.* **15**, 2470 (2024).

[8] Lu, C., Pan, Z., Yang, F. & Wu, C. Interlayer coupling driven high-temperature superconductivity in $La_3Ni_2O_7$ under pressure. Preprint at https://arxiv.org/abs/2307.14965 (2023).

[9] Zhang, Z., Greenblatt, M. & Goodenough, J. Synthesis, structure, and properties of the layered perovskite $La_3Ni_2O_{7-\delta}$. *J. Solid State Chem.* **108**, 402–409 (1994).

[10] Sahinovic, A., Geisler, B. & Pentcheva, R. Nature of the magnetic coupling in infinite-layer nickelates versus cuprates. *Phys. Rev. Mater.* **7**, 114803 (2023).
